# Supplementary material for: Can Image Generators Hold a Scene Together When Space Is Broken Apart?
Source: arXiv:2611.20906 source file (2026-11-16)
Supplement: Supplementary file 1 [file tab_flux3_captions_body.tex]

\textsc{Text} & 91 & 85\% & 81\% & 41\% \\
\textsc{Layout} & 96 & 45\% & 31\% & -- \\
\textsc{Ref} & 96 & 42\% & 91\% & 51\% \\
\textsc{Ref+Layout} & 96 & 54\% & 46\% & -- \\
