# Supplementary material for: Can Image Generators Hold a Scene Together When Space Is Broken Apart?
Source: arXiv:2611.20906 source file (2026-11-16)
Supplement: Supplementary file 2 [file tab_joint_body.tex]

GPT Image 2.6 & .37 & .44 & .49 & .33 & .38 & .43 & 1.00 & 1.00 & 1.00 & .89 & .95 & .94 \\
Nano Banana 2.1 & .36 & .44 & .47 & .32 & .37 & .40 & 1.00 & 1.00 & 1.00 & .82 & .80 & .75 \\
Muse Image 1.0 & .32 & .39 & .43 & .30 & .35 & .38 & 1.00 & 1.00 & .99 & .87 & .94 & .92 \\
Qwen-Image-2.1 & .31 & .31 & .37 & .29 & .29 & .33 & .91 & .90 & .85 & .62 & .61 & .59 \\
FLUX 3 Image Klein & .28 & .31 & .37 & .27 & .28 & .34 & .84 & .87 & .84 & .44 & .48 & .44 \\
Whole-scene control & .93 & .93 & .92 & .93 & .93 & .92 & 1.00 & 1.00 & 1.00 & 1.00 & 1.00 & 1.00 \\
\midrule
Exact cut & .91 & .91 & .90 & .91 & .91 & .90 & 1.00 & 1.00 & 1.00 & 1.00 & 1.00 & 1.00 \\
Outlines exchanged within the cut & .91 & .91 & .91 & .47 & .44 & .50 & 1.00 & 1.00 & .99 & .97 & 1.00 & .99 \\
Outlines from unrelated cuts & .90 & .91 & .91 & .90 & .72 & .75 & 1.00 & 1.00 & .99 & .25 & .92 & .88 \\
Exact cut of another scene & .34 & .42 & .47 & .31 & .38 & .42 & 1.00 & 1.00 & 1.00 & 1.00 & 1.00 & 1.00 \\
Square tiles, exact cut & -- & -- & -- & -- & -- & -- & -- & .02 & -- & -- & .00 & -- \\
