# Supplementary material for: Can Image Generators Hold a Scene Together When Space Is Broken Apart?
Source: arXiv:2611.20906 source file (2026-11-16)
Supplement: Supplementary file 3 [file tab_squares_body.tex]

GPT Image 2.6 & .97 & 1.00 & .47 & .43 & .37 & .39 & .84 & \textbf{+.16} & +.02 & \textbf{+.44} \\
Nano Banana 2.1 & .75 & .88 & .88 & .44 & .37 & .51 & .63 & \textbf{+.12} & \textbf{+.14} & \textbf{+.12} \\
Muse Image 1.0 & .81 & .78 & .97 & .40 & .33 & .36 & .85 & \textbf{+.15} & \textbf{+.03} & \textbf{+.49} \\
Qwen-Image-2.1 & .53 & .94 & .91 & .29 & .27 & .27 & .61 & \textbf{+.30} & +.00 & \textbf{+.34} \\
FLUX 3 Image Klein & .78 & .88 & .66 & .34 & .30 & .32 & .85 & \textbf{+.23} & +.02 & \textbf{+.52} \\
\midrule
Exact cut & 1.00 & 1.00 & 1.00 & .92 & .97 & .97 & .97 & & & \\
Another scene & & & & .43 & .27 & .27 & .27 & & & \\
