# Supplementary material for: Can Image Generators Hold a Scene Together When Space Is Broken Apart?
Source: arXiv:2611.20906 source file (2026-11-16)
Supplement: Supplementary file 4 [file tab_v3_bound_body.tex]

GPT Image 2.6 & .63 & 0.015 & .74 & .74 \\
Nano Banana 2.1 & .62 & 0.011 & .57 & .60 \\
Muse Image 1.0 & .51 & 0.024 & .65 & .66 \\
Qwen-Image-2.1 & .72 & 0.035 & .50 & .50 \\
FLUX 3 Image Klein & .56 & 0.029 & .33 & .35 \\
FLUX.2 [klein] & .86 & 0.103 & .04 & .07 \\
