# Supplementary material for: Can Image Generators Hold a Scene Together When Space Is Broken Apart?
Source: arXiv:2611.20906 source file (2026-11-16)
Supplement: Supplementary file 5 [file tab_v3_cells_body.tex]

GPT Image 2.6 & \textsc{Text} & 4 & 1.00 & .00 & .00 & 0.00 & .00 & .63 & -- & -- & -- & -- \\
 &  & 9 & .97 & .03 & .00 & 0.03 & .01 & .62 & -- & -- & -- & -- \\
 &  & 16 & .94 & .06 & .00 & 0.09 & .01 & .69 & -- & -- & -- & -- \\
 & \textsc{Layout} & 4 & 1.00 & .00 & .00 & 0.00 & .00 & .85 & -- & -- & -- & -- \\
 &  & 9 & .97 & .00 & .03 & 0.00 & .00 & .81 & -- & -- & -- & -- \\
 &  & 16 & .97 & .00 & .03 & 0.03 & .00 & .78 & -- & -- & -- & -- \\
 & \textsc{Ref} & 4 & 1.00 & .00 & .00 & 0.00 & .00 & .66 & .38 & .37 & .38 & .30 \\
 &  & 9 & .97 & .00 & .03 & 0.00 & .01 & .67 & .43 & .42 & .43 & .32 \\
 &  & 16 & .91 & .06 & .03 & 0.12 & .02 & .71 & .47 & .47 & .47 & .34 \\
 & \textsc{Ref+Layout} & 4 & .94 & .03 & .03 & 0.03 & .00 & .80 & .39 & .39 & .39 & .31 \\
 &  & 9 & 1.00 & .00 & .00 & 0.00 & .00 & .82 & .48 & .47 & .48 & .36 \\
 &  & 16 & .94 & .00 & .06 & 0.00 & .00 & .77 & .52 & .52 & .52 & .39 \\
\midrule
Nano Banana 2.1 & \textsc{Text} & 4 & .97 & .00 & .03 & 0.00 & .00 & .59 & -- & -- & -- & -- \\
 &  & 9 & .84 & .00 & .16 & 0.03 & .00 & .63 & -- & -- & -- & -- \\
 &  & 16 & .25 & .03 & .72 & 0.16 & .00 & .55 & -- & -- & -- & -- \\
 & \textsc{Layout} & 4 & .88 & .00 & .12 & 0.00 & .00 & .66 & -- & -- & -- & -- \\
 &  & 9 & .94 & .00 & .06 & 0.00 & .00 & .67 & -- & -- & -- & -- \\
 &  & 16 & .69 & .00 & .31 & 0.00 & .00 & .60 & -- & -- & -- & -- \\
 & \textsc{Ref} & 4 & .97 & .00 & .03 & 0.00 & .00 & .55 & .37 & .36 & .39 & .29 \\
 &  & 9 & .75 & .03 & .22 & 0.47 & .01 & .55 & .44 & .42 & .47 & .32 \\
 &  & 16 & .28 & .06 & .66 & 0.56 & .00 & .53 & .47 & .44 & .53 & .36 \\
 & \textsc{Ref+Layout} & 4 & 1.00 & .00 & .00 & 0.00 & .00 & .71 & .38 & .38 & .39 & .31 \\
 &  & 9 & .78 & .00 & .22 & 0.00 & .00 & .66 & .46 & .45 & .47 & .35 \\
 &  & 16 & .56 & .00 & .44 & 0.00 & .00 & .59 & .50 & .47 & .53 & .38 \\
\midrule
Muse Image 1.0 & \textsc{Text} & 4 & .78 & .00 & .22 & 0.00 & .04 & .46 & -- & -- & -- & -- \\
 &  & 9 & .69 & .00 & .31 & 0.00 & .01 & .57 & -- & -- & -- & -- \\
 &  & 16 & .47 & .19 & .34 & 0.03 & .01 & .58 & -- & -- & -- & -- \\
 & \textsc{Layout} & 4 & .66 & .03 & .31 & 0.03 & .07 & .71 & -- & -- & -- & -- \\
 &  & 9 & .56 & .00 & .44 & 0.06 & .02 & .75 & -- & -- & -- & -- \\
 &  & 16 & .66 & .00 & .34 & 0.16 & .01 & .71 & -- & -- & -- & -- \\
 & \textsc{Ref} & 4 & .78 & .00 & .22 & 0.03 & .05 & .45 & .33 & .31 & .35 & .31 \\
 &  & 9 & .81 & .00 & .19 & 0.03 & .02 & .56 & .40 & .39 & .42 & .33 \\
 &  & 16 & .38 & .25 & .38 & 0.06 & .01 & .61 & .44 & .43 & .46 & .35 \\
 & \textsc{Ref+Layout} & 4 & .75 & .00 & .25 & 0.00 & .05 & .63 & .32 & .31 & .34 & .30 \\
 &  & 9 & .81 & .03 & .16 & 0.03 & .02 & .69 & .39 & .38 & .40 & .31 \\
 &  & 16 & .50 & .03 & .47 & 0.19 & .01 & .69 & .44 & .42 & .45 & .34 \\
\midrule
Qwen-Image-2.1 & \textsc{Text} & 4 & .75 & .22 & .03 & 0.47 & .00 & .25 & -- & -- & -- & -- \\
 &  & 9 & .84 & .16 & .00 & 0.53 & .00 & .36 & -- & -- & -- & -- \\
 &  & 16 & .56 & .38 & .06 & 1.34 & .00 & .34 & -- & -- & -- & -- \\
 & \textsc{Layout} & 4 & .97 & .00 & .03 & 0.00 & .00 & .83 & -- & -- & -- & -- \\
 &  & 9 & .94 & .00 & .06 & 0.00 & .00 & .76 & -- & -- & -- & -- \\
 &  & 16 & .97 & .00 & .03 & 0.00 & .00 & .71 & -- & -- & -- & -- \\
 & \textsc{Ref} & 4 & .59 & .38 & .03 & 0.94 & .00 & .20 & .33 & .37 & .34 & .33 \\
 &  & 9 & .53 & .44 & .03 & 3.06 & .00 & .20 & .29 & .37 & .28 & .37 \\
 &  & 16 & .19 & .75 & .06 & 6.62 & .00 & .25 & .33 & .44 & .30 & .37 \\
 & \textsc{Ref+Layout} & 4 & .84 & .00 & .16 & 0.00 & .00 & .76 & .32 & .31 & .34 & .43 \\
 &  & 9 & .72 & .00 & .28 & 0.00 & .00 & .74 & .36 & .35 & .38 & .42 \\
 &  & 16 & .88 & .00 & .12 & 0.00 & .00 & .70 & .42 & .41 & .43 & .45 \\
\midrule
FLUX 3 Image Klein & \textsc{Text} & 4 & .78 & .16 & .06 & 0.41 & .02 & .25 & -- & -- & -- & -- \\
 &  & 9 & .62 & .19 & .19 & 0.75 & .04 & .34 & -- & -- & -- & -- \\
 &  & 16 & .50 & .34 & .16 & 2.00 & .00 & .31 & -- & -- & -- & -- \\
 & \textsc{Layout} & 4 & .62 & .22 & .16 & 0.72 & .02 & .38 & -- & -- & -- & -- \\
 &  & 9 & .59 & .19 & .22 & 1.84 & .02 & .39 & -- & -- & -- & -- \\
 &  & 16 & .69 & .19 & .12 & 2.78 & .00 & .50 & -- & -- & -- & -- \\
 & \textsc{Ref} & 4 & .75 & .19 & .06 & 0.41 & .06 & .26 & .30 & .31 & .32 & .30 \\
 &  & 9 & .78 & .16 & .06 & 1.03 & .04 & .35 & .34 & .35 & .35 & .30 \\
 &  & 16 & .19 & .38 & .44 & 3.56 & .00 & .25 & .38 & .37 & .42 & .36 \\
 & \textsc{Ref+Layout} & 4 & .75 & .19 & .06 & 0.53 & .02 & .22 & .31 & .33 & .31 & .31 \\
 &  & 9 & .69 & .22 & .09 & 1.78 & .03 & .27 & .35 & .36 & .37 & .31 \\
 &  & 16 & .19 & .56 & .25 & 5.44 & .01 & .24 & .40 & .42 & .40 & .36 \\
\midrule
FLUX.2 [klein] & \textsc{Text} & 4 & .09 & .91 & .00 & 2.62 & .06 & .03 & -- & -- & -- & -- \\
 &  & 9 & .03 & .81 & .16 & 7.94 & .00 & .02 & -- & -- & -- & -- \\
 &  & 16 & .00 & .97 & .03 & 14.91 & .02 & .02 & -- & -- & -- & -- \\
 & \textsc{Layout} & 4 & .28 & .69 & .03 & 2.19 & .02 & .12 & -- & -- & -- & -- \\
 &  & 9 & .09 & .88 & .03 & 6.22 & .02 & .07 & -- & -- & -- & -- \\
 &  & 16 & .06 & .88 & .06 & 12.69 & .02 & .06 & -- & -- & -- & -- \\
 & \textsc{Ref} & 4 & .06 & .84 & .09 & 2.78 & .05 & .04 & .25 & .36 & .28 & .40 \\
 &  & 9 & .03 & .91 & .06 & 7.94 & .00 & .01 & .22 & .44 & .21 & .44 \\
 &  & 16 & .03 & .88 & .09 & 14.94 & .00 & .02 & .19 & .44 & .17 & .54 \\
 & \textsc{Ref+Layout} & 4 & .25 & .69 & .06 & 2.50 & .05 & .05 & .32 & .42 & .29 & .39 \\
 &  & 9 & .12 & .88 & .00 & 7.12 & .06 & .05 & .33 & .47 & .31 & .41 \\
 &  & 16 & .00 & .88 & .12 & 13.16 & .03 & .05 & .31 & .46 & .30 & .40 \\
