# Supplementary material for: Can Image Generators Hold a Scene Together When Space Is Broken Apart?
Source: arXiv:2611.20906 source file (2026-11-16)
Supplement: Supplementary file 6 [file tab_v3_constructions_body.tex]

Exact cut & .95 & .93 & .88 & .92 & .92 & .92 & .92 & .92 & .92 & .92 & .92 & .92 \\
One piece missing & .63 & .85 & .84 & .79 & .86 & .89 & .92 & .92 & .92 & .69 & .82 & .86 \\
Three pieces missing & .00 & .77 & .79 & .38 & .73 & .82 & .88 & .91 & .90 & .24 & .61 & .76 \\
One piece duplicated & .95 & .93 & .88 & .81 & .87 & .89 & .81 & .87 & .89 & .81 & .87 & .89 \\
Half the pieces duplicated & .95 & .93 & .88 & .70 & .77 & .77 & .70 & .77 & .77 & .70 & .77 & .77 \\
One piece from another scene & .95 & .93 & .88 & .77 & .86 & .89 & .77 & .86 & .89 & .77 & .86 & .89 \\
Half the pieces from another scene & .95 & .93 & .88 & .62 & .69 & .67 & .62 & .69 & .67 & .62 & .69 & .67 \\
Outlines exchanged within the cut & .94 & .93 & .87 & .93 & .92 & .92 & .93 & .92 & .92 & .93 & .92 & .92 \\
Each outline from an unrelated cut & .24 & .86 & .76 & .92 & .92 & .92 & .92 & .92 & .92 & .92 & .92 & .92 \\
Content turned $2^\circ$ & .95 & .93 & .88 & .82 & .87 & .88 & .82 & .87 & .88 & .82 & .87 & .88 \\
Content turned $5^\circ$ & .95 & .93 & .88 & .67 & .75 & .80 & .67 & .75 & .80 & .67 & .75 & .80 \\
Content turned $10^\circ$ & .95 & .93 & .88 & .55 & .65 & .70 & .55 & .65 & .70 & .55 & .65 & .70 \\
Content turned $20^\circ$ & .95 & .93 & .88 & .45 & .55 & .61 & .45 & .55 & .61 & .45 & .55 & .61 \\
Content turned $45^\circ$ & .95 & .93 & .88 & .39 & .49 & .55 & .39 & .49 & .55 & .39 & .49 & .55 \\
Content scaled $\times0.9$ & .95 & .93 & .88 & .63 & .72 & .76 & .63 & .72 & .76 & .63 & .72 & .76 \\
Content scaled $\times0.75$ & .95 & .93 & .88 & .48 & .57 & .63 & .48 & .57 & .63 & .48 & .58 & .63 \\
Content scaled $\times0.5$ & .95 & .93 & .88 & .36 & .46 & .52 & .36 & .45 & .52 & .37 & .47 & .52 \\
Content scaled $\times1.25$ & .95 & .93 & .88 & .54 & .62 & .69 & .54 & .62 & .69 & .54 & .62 & .69 \\
Content scaled $\times1.5$ & .95 & .93 & .88 & .47 & .56 & .62 & .47 & .56 & .62 & .47 & .56 & .62 \\
Pieces cut from a $2\times$ zoom & .95 & .93 & .88 & .39 & .48 & .54 & .38 & .48 & .53 & .40 & .49 & .54 \\
Pieces cut from a $3\times$ zoom & .95 & .93 & .87 & .40 & .49 & .53 & .39 & .48 & .52 & .41 & .50 & .55 \\
Every piece a thumbnail & .95 & .94 & .88 & .33 & .36 & .39 & .33 & .35 & .39 & .33 & .36 & .39 \\
Exact cut of another scene & .95 & .93 & .88 & .35 & .43 & .48 & .35 & .43 & .47 & .35 & .43 & .49 \\
