# Supplementary material for: Can Image Generators Hold a Scene Together When Space Is Broken Apart?
Source: arXiv:2611.20906 source file (2026-11-16)
Supplement: Supplementary file 7 [file tab_v3_contrast_ci_body.tex]

GPT Image 2.6 & +.01 [$-$.02, .03] & +.14 [.12, .16] & +.04 [.03, .05] & $-$.02 [$-$.05, .02] & +.01 [$-$.01, .03] \\
Nano Banana 2.1 & +.13 [.06, .21] & +.08 [.06, .10] & +.02 [.01, .03] & $-$.04 [$-$.11, .04] & $-$.02 [$-$.05, .01] \\
Muse Image 1.0 & +.01 [$-$.09, .10] & +.16 [.13, .18] & $-$.01 [$-$.02, .00] & +.04 [$-$.05, .14] & $-$.03 [$-$.05, $-$.01] \\
Qwen-Image-2.1 & +.31 [.23, .39] & +.48 [.46, .51] & +.05 [.02, .08] & $-$.21 [$-$.29, $-$.14] & $-$.06 [$-$.09, $-$.04] \\
FLUX 3 Image Klein & $-$.02 [$-$.10, .07] & +.04 [$-$.01, .08] & +.01 [$-$.02, .03] & $-$.08 [$-$.16, .01] & $-$.10 [$-$.13, $-$.06] \\
FLUX.2 [klein] & +.09 [.04, .15] & +.04 [.03, .05] & +.10 [.07, .13] & $-$.01 [$-$.07, .06] & $-$.02 [$-$.04, $-$.00] \\
