# Supplementary material for: Can Image Generators Hold a Scene Together When Space Is Broken Apart?
Source: arXiv:2611.20906 source file (2026-11-16)
Supplement: Supplementary file 8 [file tab_v3_main_ci_body.tex]

GPT Image 2.6 & 4 & .98 [.96, 1.00] & .74 [.71, .76] & .38 [.34, .42] \\
 & 9 & .98 [.95, 1.00] & .73 [.71, .74] & .45 [.41, .49] \\
 & 16 & .94 [.90, .97] & .74 [.73, .75] & .49 [.46, .53] \\
\addlinespace
Nano Banana 2.1 & 4 & .95 [.91, .98] & .63 [.60, .66] & .38 [.34, .41] \\
 & 9 & .83 [.76, .89] & .63 [.61, .64] & .45 [.42, .49] \\
 & 16 & .45 [.37, .52] & .57 [.55, .58] & .48 [.45, .51] \\
\addlinespace
Muse Image 1.0 & 4 & .74 [.66, .82] & .56 [.53, .60] & .33 [.29, .36] \\
 & 9 & .72 [.64, .79] & .64 [.62, .66] & .40 [.36, .43] \\
 & 16 & .50 [.42, .58] & .65 [.63, .67] & .44 [.40, .48] \\
\addlinespace
Qwen-Image-2.1 & 4 & .79 [.72, .86] & .51 [.49, .53] & .33 [.30, .36] \\
 & 9 & .76 [.69, .83] & .51 [.49, .54] & .33 [.29, .36] \\
 & 16 & .65 [.59, .70] & .50 [.48, .52] & .37 [.33, .41] \\
\addlinespace
FLUX 3 Image Klein & 4 & .73 [.65, .79] & .28 [.23, .32] & .31 [.27, .34] \\
 & 9 & .67 [.57, .76] & .34 [.29, .38] & .35 [.30, .38] \\
 & 16 & .39 [.31, .48] & .33 [.28, .37] & .39 [.35, .43] \\
\addlinespace
FLUX.2 [klein] & 4 & .17 [.11, .23] & .06 [.04, .08] & .29 [.25, .32] \\
 & 9 & .07 [.03, .12] & .04 [.03, .05] & .28 [.24, .31] \\
 & 16 & .02 [.00, .05] & .04 [.03, .05] & .25 [.22, .29] \\
