# Supplementary material for: Can Image Generators Hold a Scene Together When Space Is Broken Apart?
Source: arXiv:2611.20906 source file (2026-11-16)
Supplement: Supplementary file 9 [file tab_v3_readings_body.tex]

GPT Image 2.6 & A & .95 & .89 & .81 & .67 & .64 & .62 & .36 & .43 & .47 \\
 & B & .98 & .90 & .82 & .70 & .66 & .66 & .38 & .45 & .49 \\
 & C & .87 & .77 & .65 & .68 & .66 & .65 & .35 & .42 & .45 \\
 & D & .80 & .69 & .60 & .71 & .71 & .71 & .36 & .43 & .47 \\
\addlinespace
Nano Banana 2.1 & A & .95 & .80 & .41 & .54 & .53 & .44 & .35 & .41 & .44 \\
 & B & .93 & .80 & .38 & .54 & .53 & .44 & .35 & .42 & .45 \\
 & C & .65 & .42 & .25 & .56 & .57 & .51 & .33 & .41 & .43 \\
 & D & .65 & .44 & .25 & .57 & .58 & .52 & .35 & .43 & .44 \\
\addlinespace
Muse Image 1.0 & A & .66 & .66 & .42 & .51 & .56 & .49 & .30 & .36 & .39 \\
 & B & .57 & .65 & .38 & .52 & .58 & .53 & .30 & .37 & .39 \\
 & C & .43 & .48 & .30 & .52 & .59 & .59 & .31 & .38 & .42 \\
 & D & .38 & .45 & .26 & .53 & .61 & .62 & .31 & .38 & .43 \\
\addlinespace
Qwen-Image-2.1 & A & .68 & .65 & .59 & .41 & .41 & .36 & .27 & .26 & .28 \\
 & B & .68 & .66 & .59 & .42 & .42 & .37 & .27 & .27 & .29 \\
 & C & .62 & .56 & .43 & .49 & .49 & .47 & .31 & .31 & .36 \\
 & D & .57 & .57 & .40 & .49 & .50 & .49 & .31 & .32 & .37 \\
\addlinespace
FLUX 3 Image Klein & A & .55 & .48 & .29 & .21 & .23 & .21 & .26 & .29 & .31 \\
 & B & .52 & .38 & .30 & .21 & .23 & .21 & .26 & .29 & .32 \\
 & C & .49 & .48 & .27 & .25 & .30 & .29 & .28 & .30 & .36 \\
 & D & .41 & .36 & .19 & .25 & .31 & .31 & .27 & .31 & .37 \\
\addlinespace
FLUX.2 [klein] & A & .06 & .01 & .00 & .03 & .02 & .01 & .19 & .16 & .15 \\
 & B & .05 & .01 & .00 & .02 & .02 & .01 & .18 & .16 & .14 \\
 & C & .08 & .03 & .01 & .04 & .03 & .02 & .25 & .23 & .22 \\
 & D & .09 & .05 & .02 & .04 & .03 & .03 & .24 & .23 & .19 \\
