# Supplementary material for: Can Image Generators Hold a Scene Together When Space Is Broken Apart?
Source: arXiv:2611.20906 source file (2026-11-16)
Supplement: Supplementary file 10 [file tab_v3_solver_body.tex]

GPT Image 2.6 & 1.00 & -- & 1.00 & -- & .63 & 0.012 \\
Nano Banana 2.1 & 1.00 & -- & 1.00 & -- & .62 & 0.008 \\
Muse Image 1.0 & 1.00 & -- & 1.00 & -- & .51 & 0.021 \\
Qwen-Image-2.1 & 1.00 & -- & 1.00 & -- & .72 & 0.028 \\
FLUX 3 Image Klein & 1.00 & -- & 1.00 & -- & .56 & 0.022 \\
FLUX.2 [klein] & 1.00 & -- & 1.00 & -- & .86 & 0.069 \\
Controls & 1.00 & -- & 1.00 & -- & 1.00 & -- \\
